# Supplementary material for: OmniOPSD: Rationale-Privileged On-Policy Self-Distillation for Affective Computing
Source: arXiv:2606.15920 source file (2026-11-05)
Supplement: Supplementary file 1 [file 7_appendix.tex]

\section{Appendix}

\subsection{Additional Details}

Additional implementation details, prompt templates, rationale-generation protocols, and extended results will be included here as they are finalized.
